# Supplementary material for: Multi-Task Recommendations with Reinforcement Learning
Source: arXiv:2302.03328 source file (2023-03-10)
Supplement: Supplementary file 1 [file 6.Appendix.tex]

\begin{appendix}

\section{Algorithm} \label{Appendixal}
To be specific, we first initialize the estimation actor-critic network and the target network. Set up the session MDP environment and sample batch of sequences from replay buffer $\mathcal{B}$ with size $b$ (line 2-7). Then, forward the target actor network to get the next action pairs $(a_{1,t+1},a_{2,t+1})$ (line 8) and calculate the action value estimator $Q(s_{t+1},a_{k,t+1}; \widetilde{\mathbf{\phi}}_k)$ and $Q(s_t,a_{k,t}; \mathbf{\phi}_k))$ for getting average TD error $\delta$ (line 9). The estimation actor-network parameters are updated based on gradients (lines 10-14). Finally, the target network parameters are soft updated (lines 16-17).

\begin{algorithm}[ht]
\caption{RL-enhanced Multi-task Learning}
\label{alg:ddpg-esmm}
{\bf Input}: Differentiable policy network $\pi(s_t; \boldsymbol{\theta})$ with the same structure as ESMM, two differentiable action value networks $Q(s_t,a_{1,t}; \mathbf{\phi}_1)$,$Q(s_t,a_{2,t}; \mathbf{\phi}_2)$. Make copies of the three as target networks $\pi(s_t; \boldsymbol{\widetilde{\theta}})$ and $Q(s_t,a_{k,t}; \mathbf{\widetilde{\phi}}_k), k=1,2$. \\
{\bf Parameters}: Learning rate $\alpha^{\mathbf{\theta}} > 0$,$\alpha^{\mathbf{\phi}} > 0$, soft update rate $\beta$, critic converge threshold $\epsilon$, polish variable $\lambda$. \\
\begin{algorithmic}[1]
\FOR{$epoch=1,2,\cdots$}
%        \STATE Sample a batch data from replay buffer $\mathcal{B}$ with size $b$
    \STATE Reset the starting state $s_t$ of the environment
    \WHILE{$s$ not terminated}
        \STATE Forward estimation actor network to get the action $a_{1,t},a_{2,t} = \pi(s_t; \boldsymbol{\theta})$;
        \STATE Perform action $a$, observe next state $s_{t+1}$ and reward $r_{1,t},r_{2,t}$;
        \STATE Store the transition $(s_t,a_{1,t},a_{2,t},s_{t+1},r_{1,t},r_{2,t})$ into replay buffer $\mathcal{B}$;
        \FOR{batch $b$ in replay buffer $\mathcal{B}$}
        \STATE Forward target actor network to get the next action $a_{1,t+1},a_{2,t+1} = \pi(s_{t+1}; \mathbf{\widetilde{\boldsymbol{\theta}}})$;
        \STATE $\delta \leftarrow \frac{1}{2b} \sum\limits_{(s,a,s',r)\in b} \sum\limits_k (r_k + \gamma Q(s',a'_k; \widetilde{\phi}_k)-Q(s,a_k; \mathbf{\phi}_k))$, \quad\quad ($Q(s',a'_k; \widetilde{\mathbf{\phi}}_k) = 0$ if $s'$ is done)

        \STATE Update $\mathbf{\phi}_k \leftarrow \mathbf{\phi}_k - \alpha^{\mathbf{\phi}}\mathbf{I}\delta \nabla_{\mathbf{\phi}}Q(s_t,a_{k,t}; \mathbf{\phi}_k)$

        \IF{$\delta \geq \epsilon$}
            \STATE $\mathbf{\theta}_k \leftarrow \mathbf{\theta}_k - \alpha^{\mathbf{\theta}}\mathbf{I} \nabla_{\mathbf{\theta}} 
            [\frac{1}{b}\sum\limits_{(s,a,s',r)\in b} Q(s_t,\pi(s_t; \mathbf{\theta}_k))]$
        \ELSE
            \STATE $\mathcal{L}(\boldsymbol{\theta}) 
                    = \sum\limits_{(s,a,s',r)\in b} \sum\limits_k {\omega_{k,t} BCE(\pi(s_t; \mathbf{\theta}_k),y_{k,t}))}$ 
                    \newline
                    $\mathbf{\theta}_k \leftarrow \mathbf{\theta}_k - \alpha^{\mathbf{\theta}}\mathbf{I} \nabla_{L(\mathbf{\theta})}$
        \ENDIF
        
        \STATE $\widetilde{\theta}_i \leftarrow \beta \widetilde{\theta}_i + (1-\beta)\theta_i $
        \STATE $\widetilde{\phi}_i \leftarrow \beta \widetilde{\phi}_i + (1-\beta)\phi_i $
        \ENDFOR
    \ENDWHILE
\ENDFOR
\end{algorithmic}
\end{algorithm}

\section{Datasets} \label{A}
\begin{itemize}[leftmargin=*]
    \item \textbf{RetailRocket} \footnote{https://www.kaggle.com/datasets/retailrocket/ecommerce-dataset} is collected from a real-world e-commerce website. It contains 1407580 user sessions of viewing and adding to cart (which corresponds to click and pay). As to the massive item properties, We do feature selection using Gini Impurity and keep the top 7 properties with respect to the device capacity. We then delete the items without complete properties and also eliminate 20\% of the long-tail categorical labels into a single group. The statistics of these two datasets are given in Table \ref{tab:dbrt-stat}. 
    \item \textbf{Kuairand-1K} \footnote{https://kuairand.com/} consists of unbiased sequential recommendation data from the logs of the short video platform application, Kuaishou. We randomly sample 300 users from the original ``Kuairand-1K'' dataset and reorganize the dataset into the session-wise format. Feature selection is conducted using Gini Impurity and keeps the top 6 properties for both user and item. The session is defined as sequential user behaviors in specific time windows sorted by timestamp, where our dataset contains 424068 user sessions. We define the click behavior by a binary feedback signal in the following rule: ``click'' = 1 when the user play duration is greater than 30 \% of video duration. We define the convert behavior by a binary feedback signal in the following rule: ``convert'' = 1 when the user play duration is greater than 70 \% of video duration.
\end{itemize}
\begin{table}[t]
    \scriptsize
    \centering
    \footnotesize
    \caption{Datasets Statistics}
    \begin{tabular}{cccccc}
    \toprule
    Dataset & \# sessions & \# interactions & \# items & \# clicks & \# converts \\
    \midrule
    RetailRocket & 1404526 & 2684433 & 234843 & 138928 & 20121 \\
    \midrule
    Kuairand & 424068 & 2387756 & 1201513 & 954913 & 669118 \\
    \bottomrule
    \end{tabular}
    \label{tab:dbrt-stat}
\end{table}

\section{Hyper-parameter selection} \label{HPS}
Hyper-parameter selection is one of the most essential steps influencing the experiment result. We choose several hyper-parameters for baseline MTL models and the RMTL model. The result is based on the average performance of each model on two datasets. And we set the number of layers for the feature MLP as 2 and set the number of layers for the tower layer as 3. The detail of hyper-parameter selection is shown in Table. \ref{table:ht}

\begin{table*}[t]
        \large
	\caption{Hyper-parameters selection result.}
	\vspace{-3mm}
	\label{table:ht}
	\begin{tabular}{@{}|c|c|c|c|@{}}
		\toprule[1pt]
		\multirow{1}{*}{Model} & \multirow{1}{*}{Hyper-parameter} & \multirow{1}{*}{Tuning range} & \multirow{1}{*}{Our choice} \\  \midrule

            \multirow{3}{*}{Baseline MTL}  
            & embedding dimension & [32,64,96,128] & 128 \\

            & dropout rate & [0,0.2,0.4,0.5,0.6] & 0.2 \\
            
            & number of expert & [4,6,8,10] & 8 \\ \midrule

            \multirow{3}{*}{RMTL} 
            & soft update rate $\beta$ & [0,0.2,0.4,0.6] & 0.2 \\

            & learning rate $\alpha^{\theta}$ & [0.05, 0.01, 0.005, 0.001, 0.0005] & 0.001 \\

            & learning rate $\alpha^{\phi}$ & [0.05, 0.01, 0.005, 0.001, 0.0005] & 0.001 \\

            & polish variable $\lambda$ & [0.1, 0.3, 0.5, 0.7, 0.9] & 0.7 \\ \midrule
	\end{tabular}
	\vspace{-5mm}
\end{table*}

\section{Transferability results} \label{B}
The transferability study for the RMTL method for the CTR task on the Kuairand dataset is shown in Figure~\ref{figure:B}.

\begin{figure}[ht]
        \Description{Transferability study results for ESMM, MMOE, and PLE on the Kuairand dataset.}
	\centering
	%	\hspace*{-0.6cm}
	{\subfigure{\includegraphics[width=0.327\linewidth]{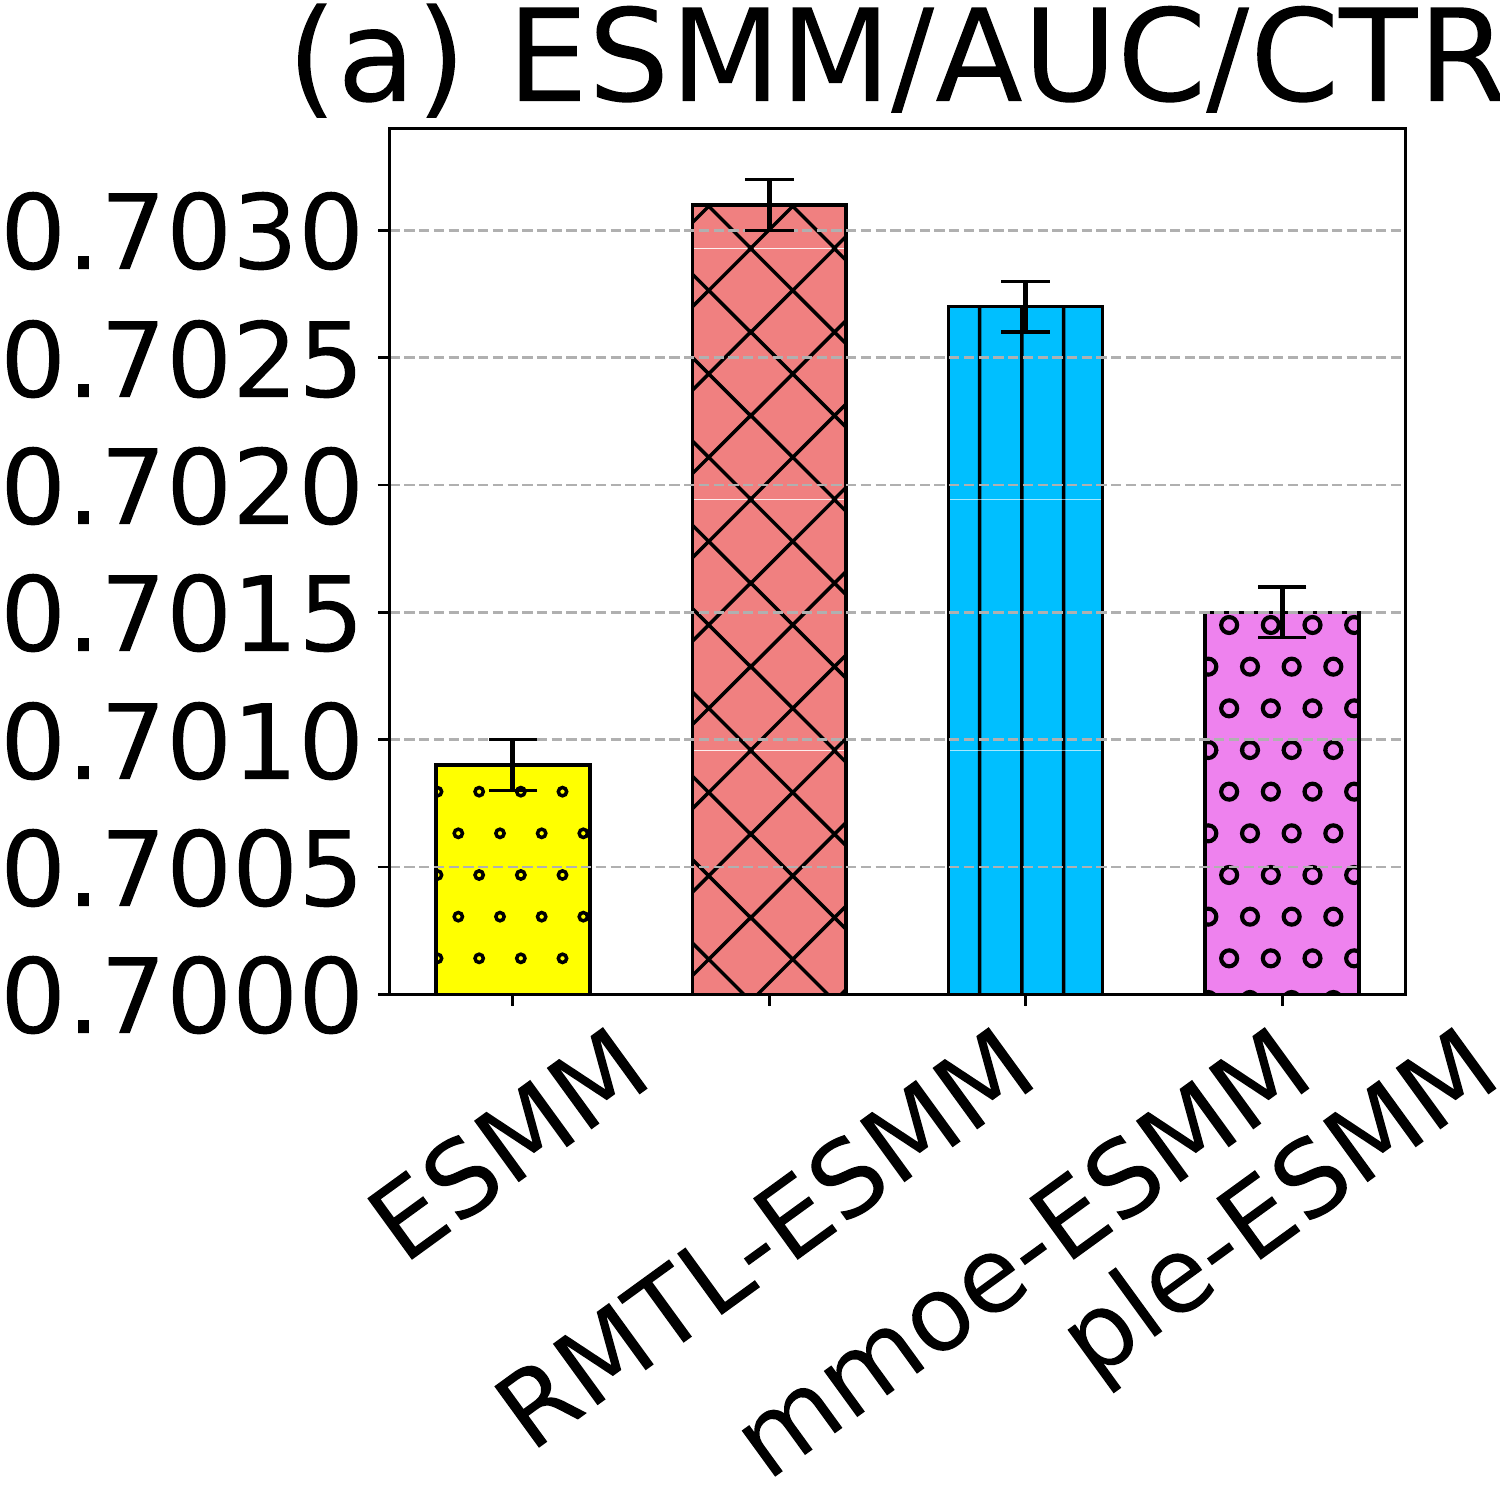}}}
	{\subfigure{\includegraphics[width=0.327\linewidth]{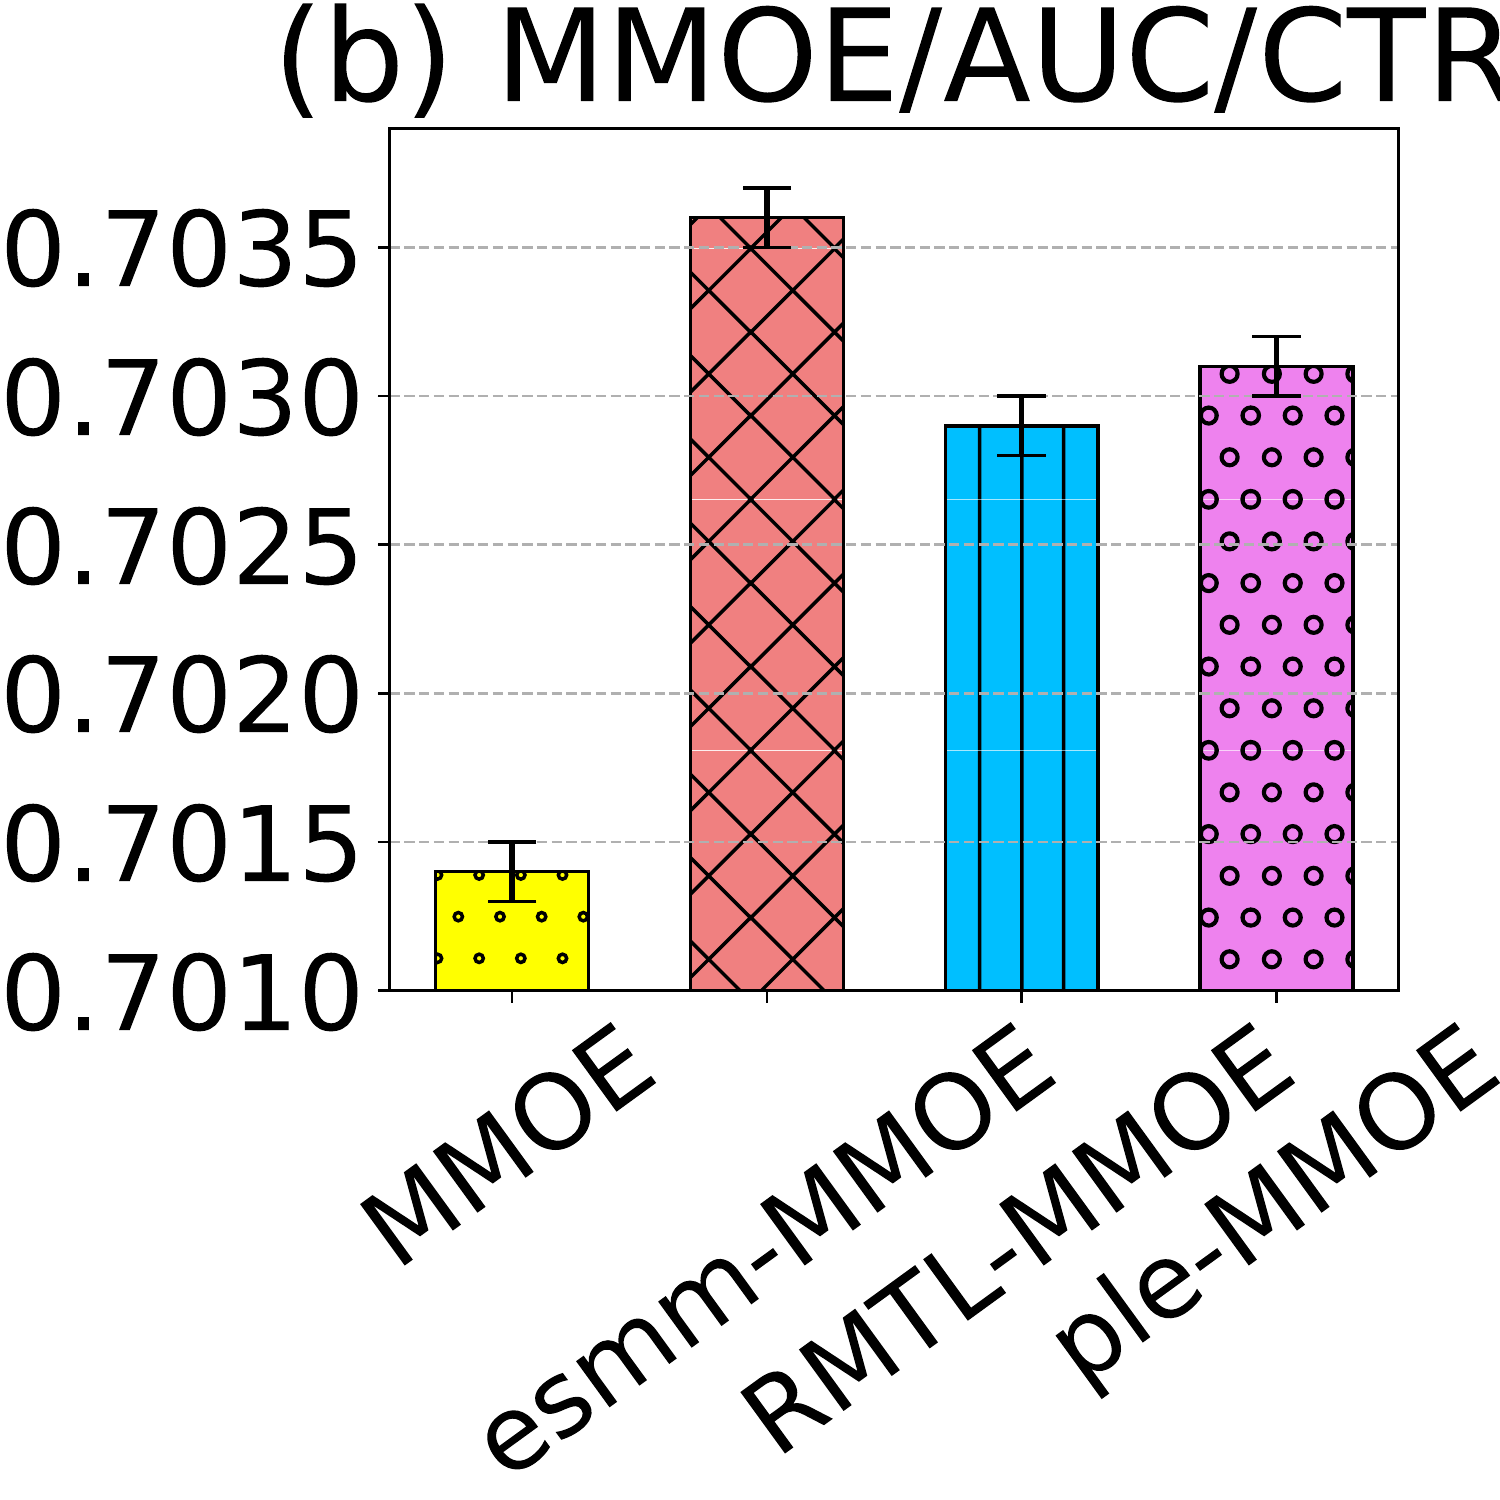}}}
	{\subfigure{\includegraphics[width=0.327\linewidth]{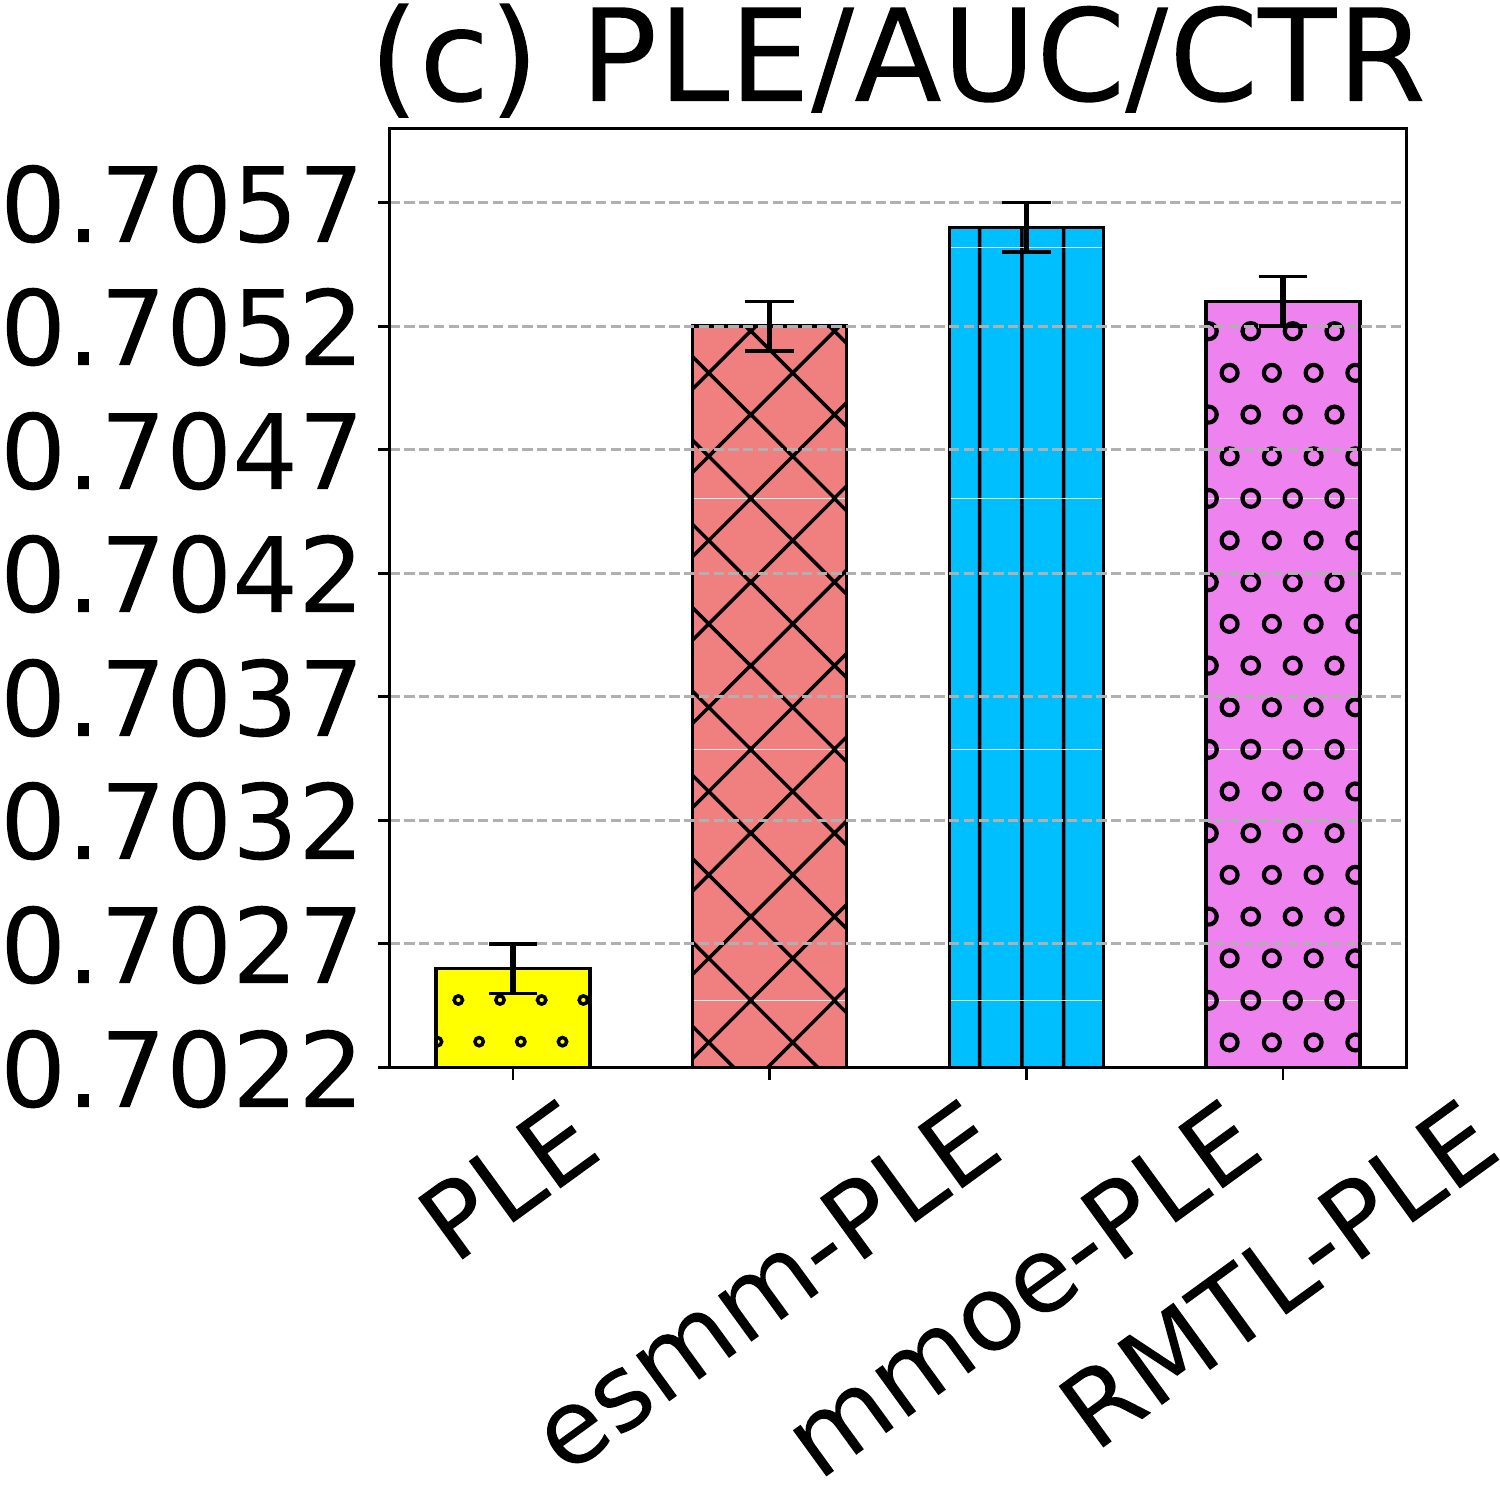}}}
	%	\hspace*{-0.6cm}
	{\subfigure{\includegraphics[width=0.327\linewidth]{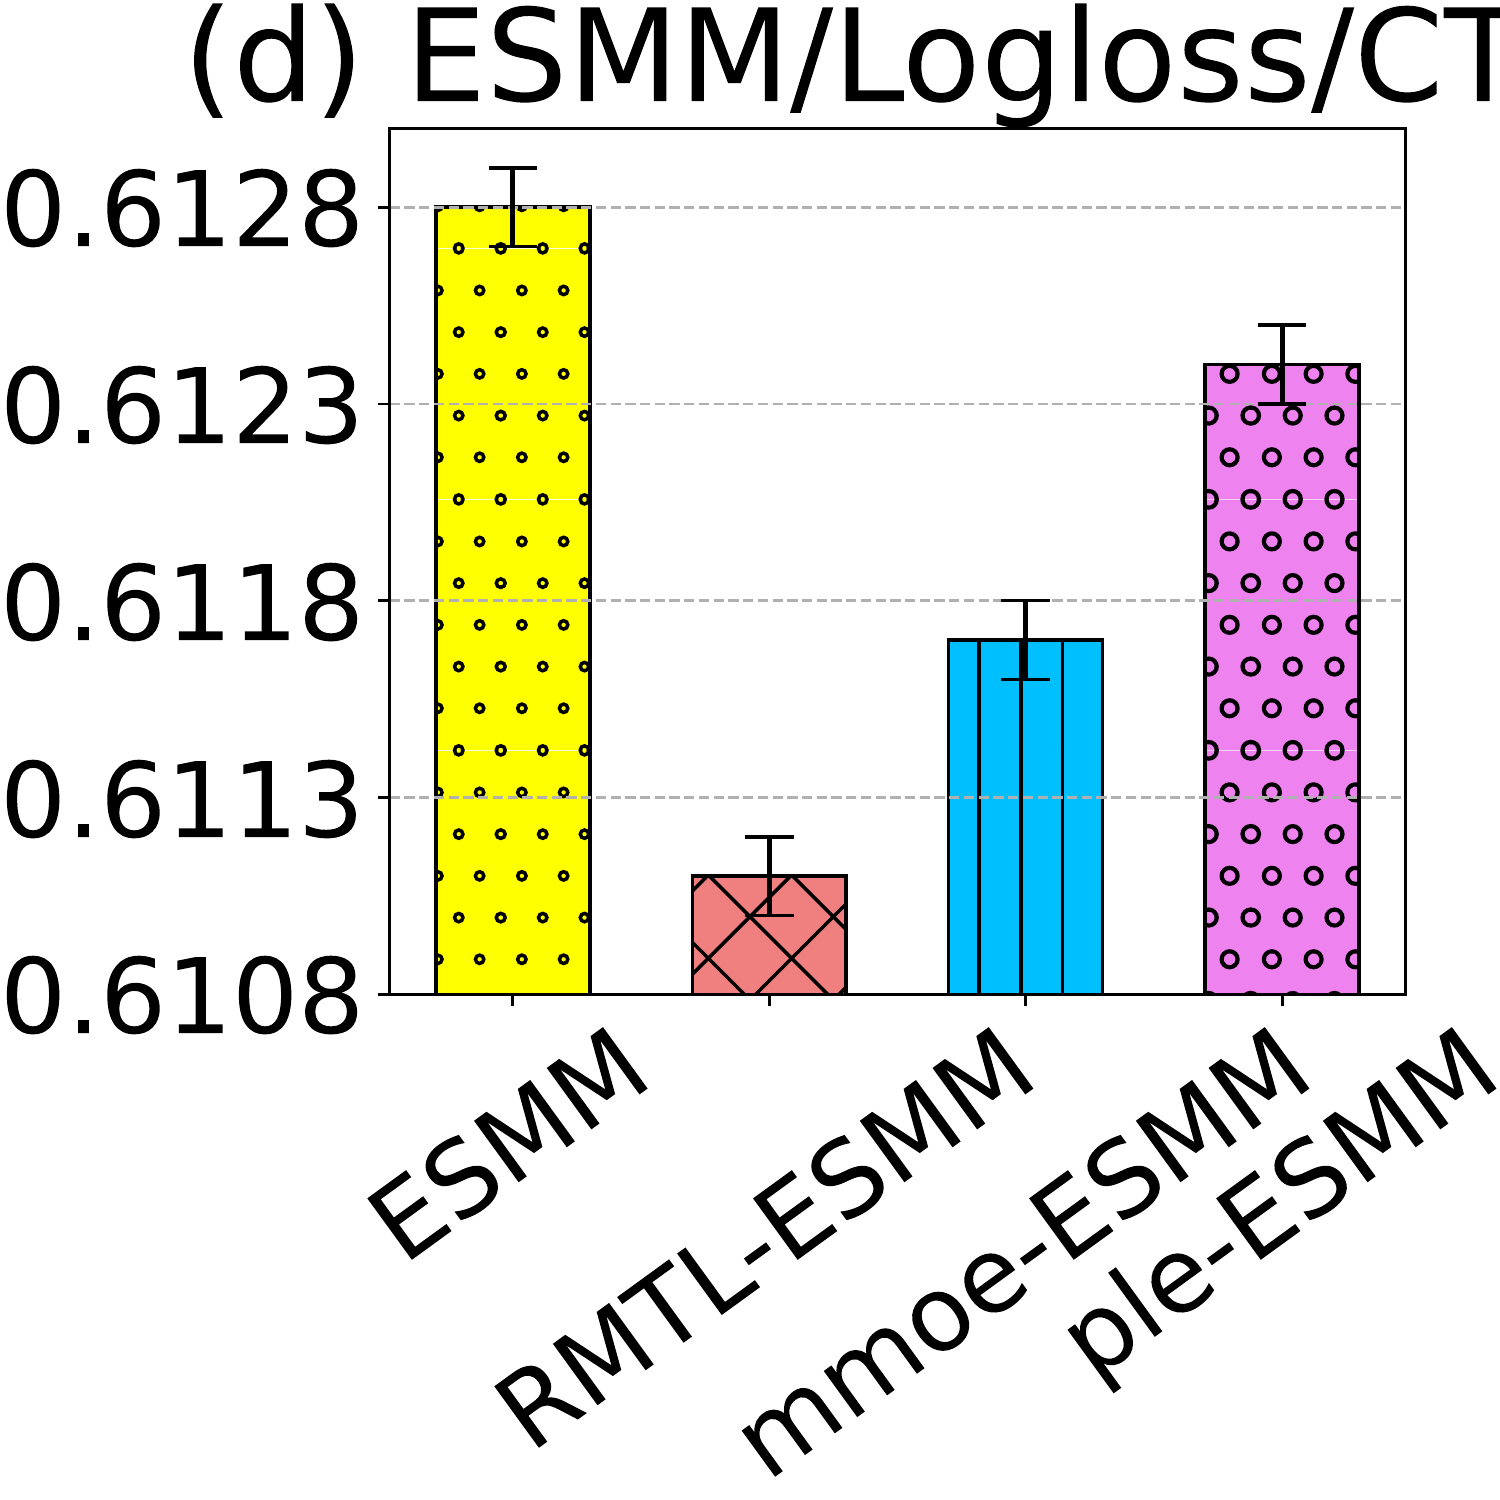}}}
	{\subfigure{\includegraphics[width=0.327\linewidth]{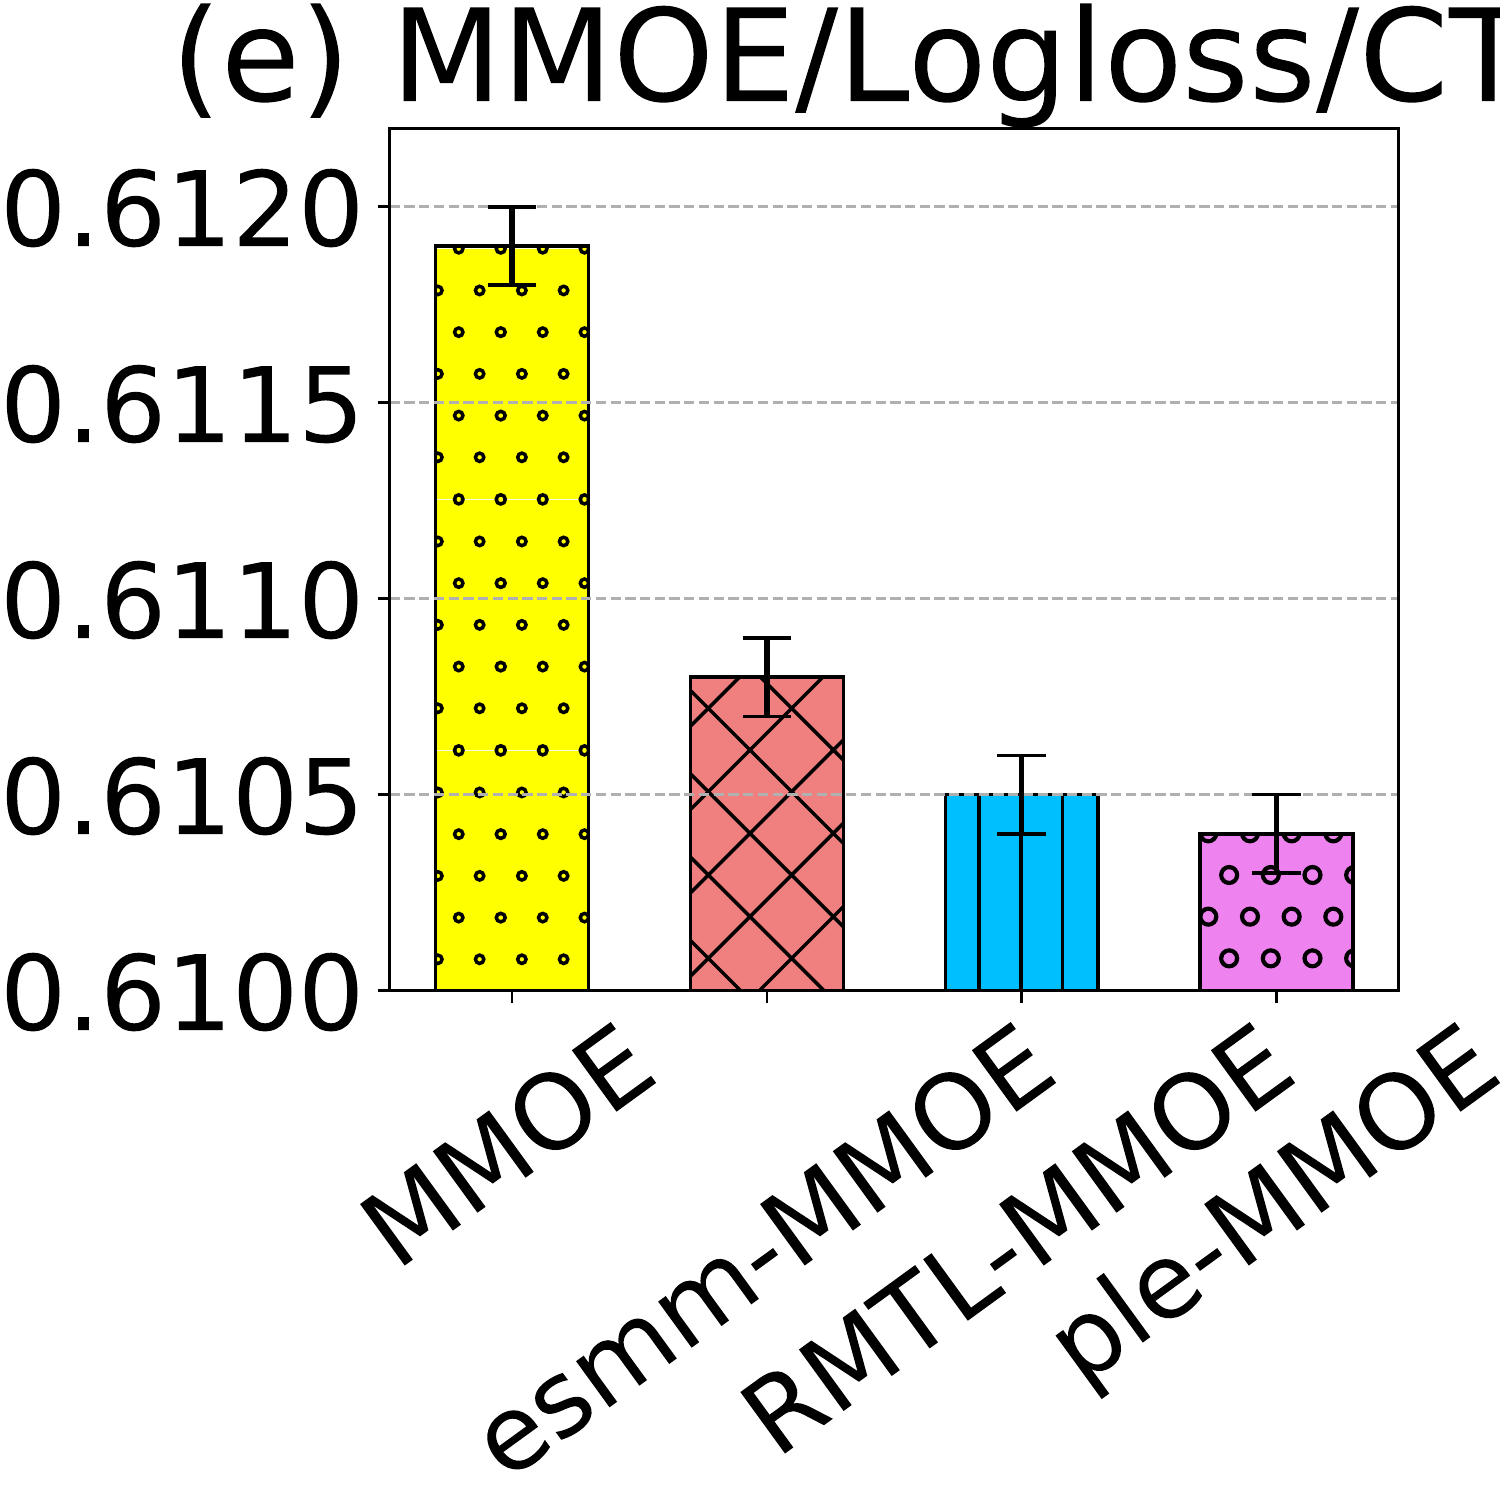}}}
	{\subfigure{\includegraphics[width=0.327\linewidth]{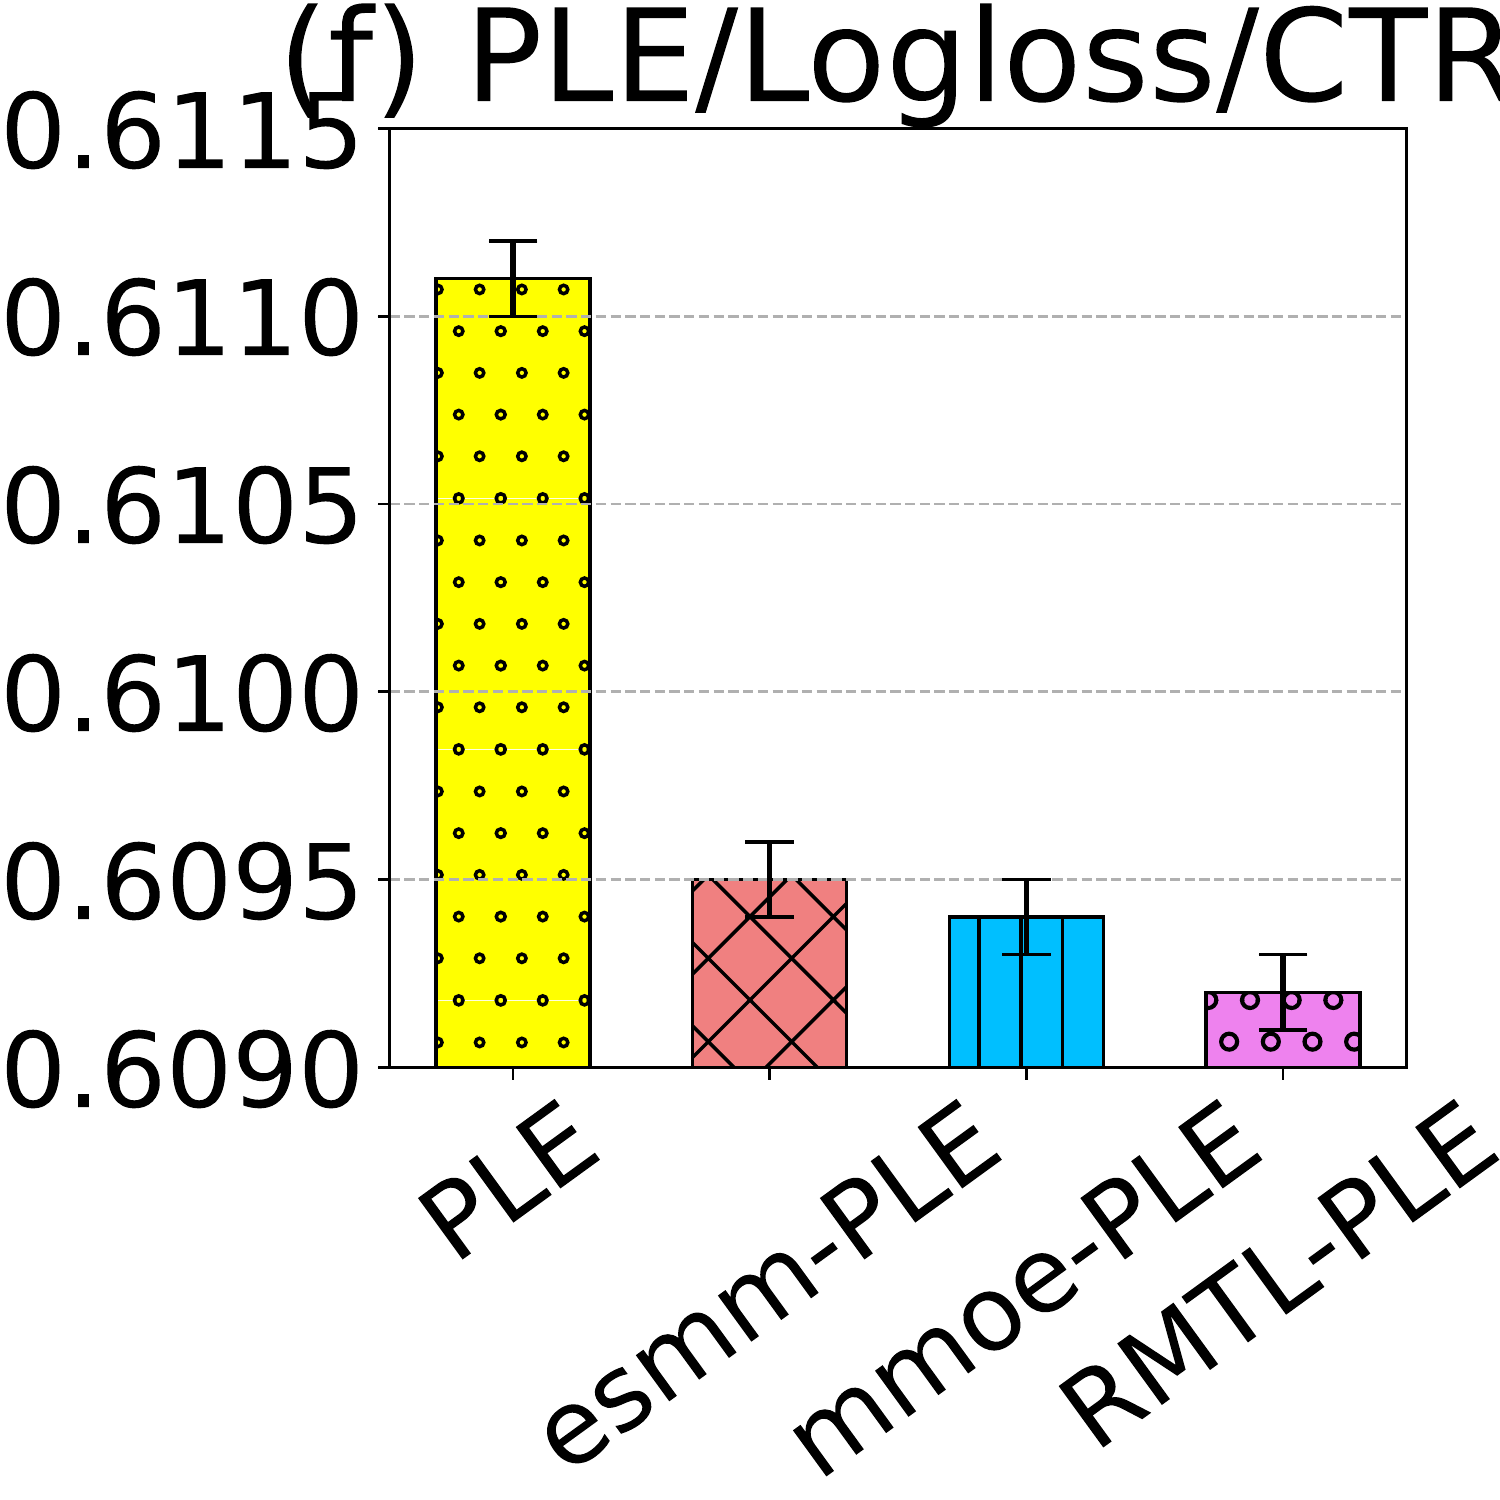}}}
	\caption{Transferability study results for Kuairand.}\label{figure:B}.
	\vspace{-4.9mm}
\end{figure}

\section{Parameter analysis} \label{AppendixC}
The analysis result of $\lambda$ is shown in Figure \ref{fig:Fig4} (a)-(d), it can be observed that:
(i) From the results of the first two figures, for the CTR prediction task, the RMTL-PLE model with $\lambda=0.3$ achieves the worst performance on both AUC and logloss metrics, while the RMTL-PLE model with $\lambda=0.7$ achieves comprehensively best performance.
(ii) From the results of the last two figures, for the CTCVR prediction task, the RMTL-PLE model with $\lambda=0.3$ achieves the best performance on AUC but the worst performance on logloss, while the RMTL-PLE model with $\lambda=0.7$ also achieves comprehensively best performance.
To summarize, the best setting of the polish variable may be $\lambda=0.7$, which outperforms other settings on both metrics.

We also conduct hyper-parameter analysis for learning rate $\alpha^{\theta}$ and $\alpha^{\phi}$ on the RetailRocket dataset, the result is shown in Table \ref{table:C1} and Table \ref{table:C2}.

\begin{figure}[h]
        \Description{Parameter analysis for $\lambda$ respect to CTR/CTCVR task and AUC/logloss metrics.}
	\centering
	%	\hspace*{-0.6cm}
	{\subfigure{\includegraphics[width=0.48\linewidth]{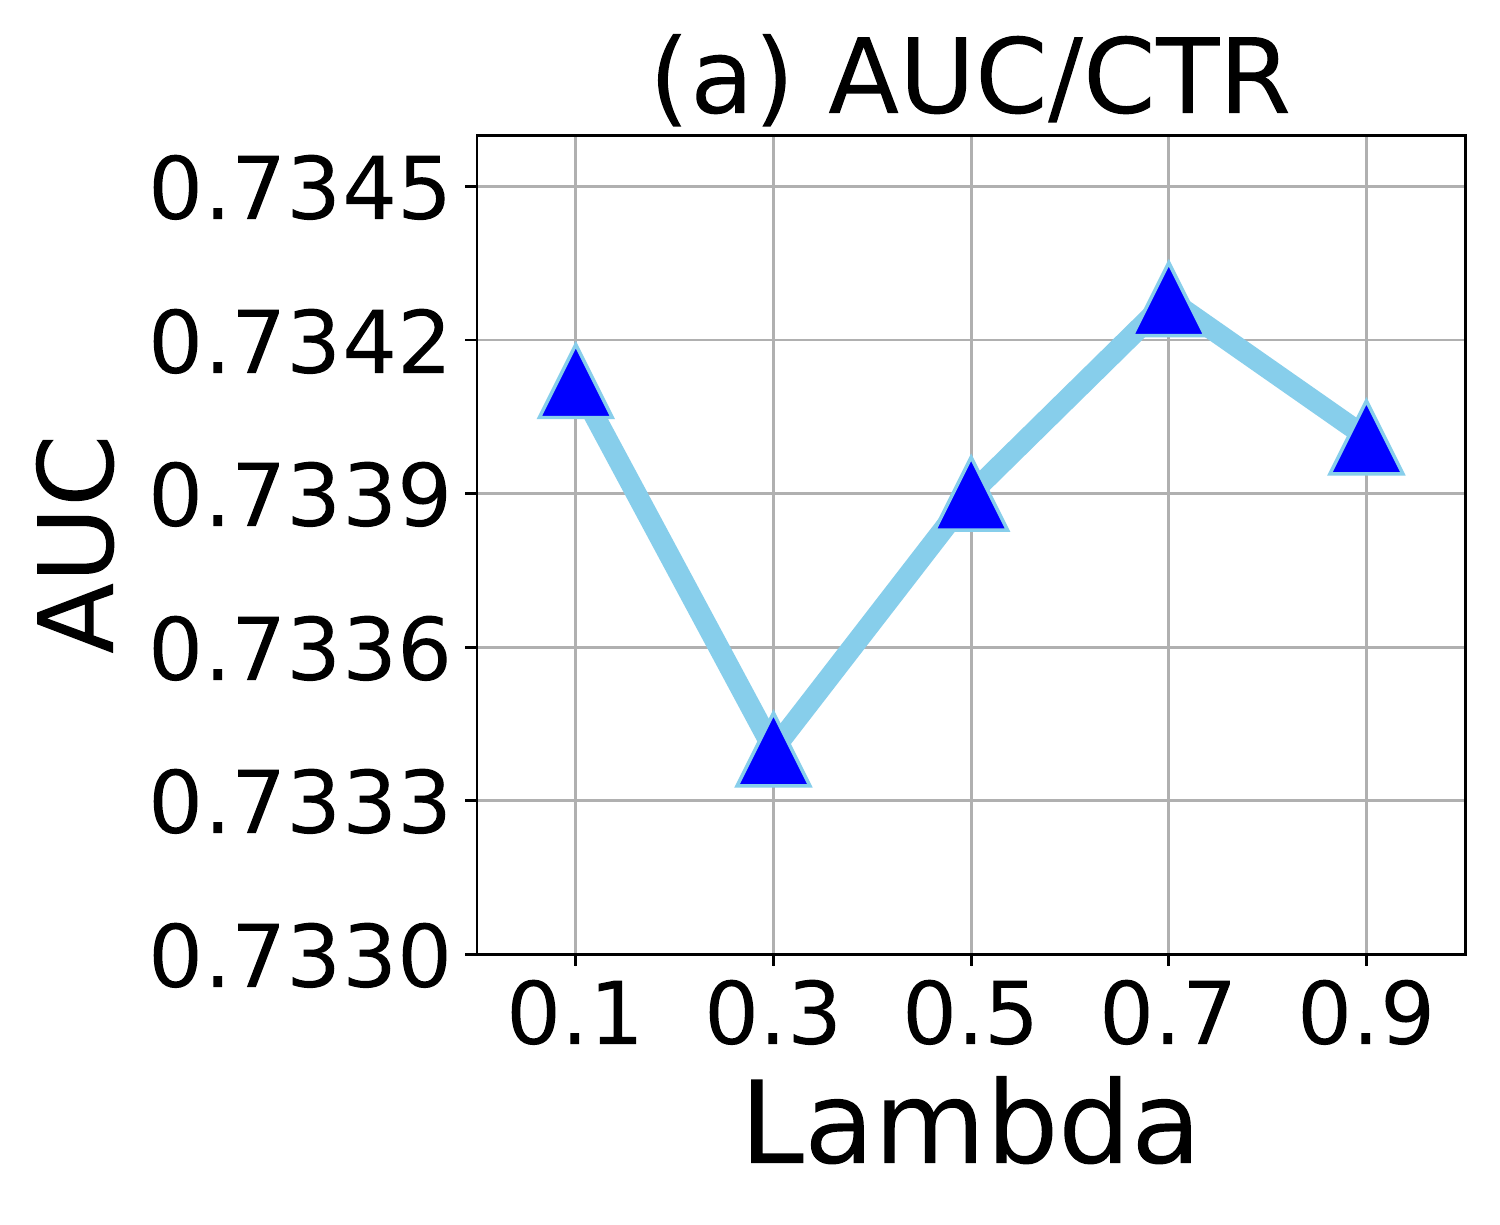}}}
	{\subfigure{\includegraphics[width=0.48\linewidth]{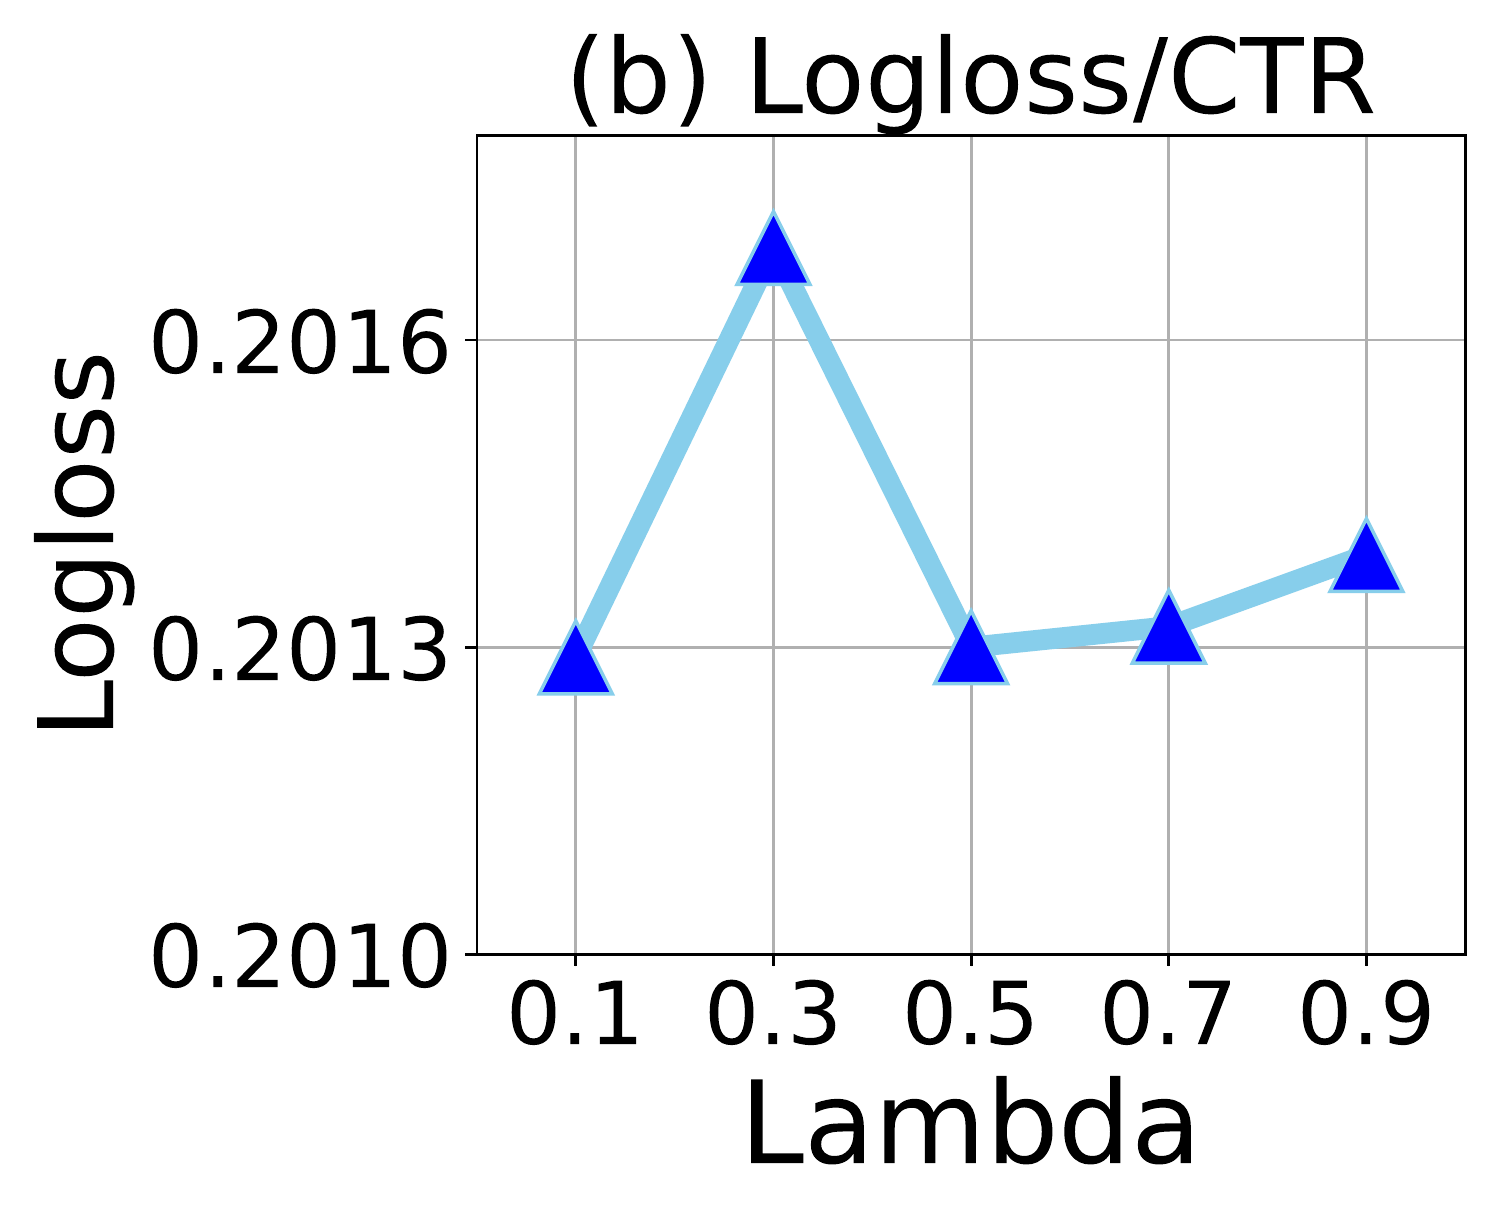}}}
	{\subfigure{\includegraphics[width=0.48\linewidth]{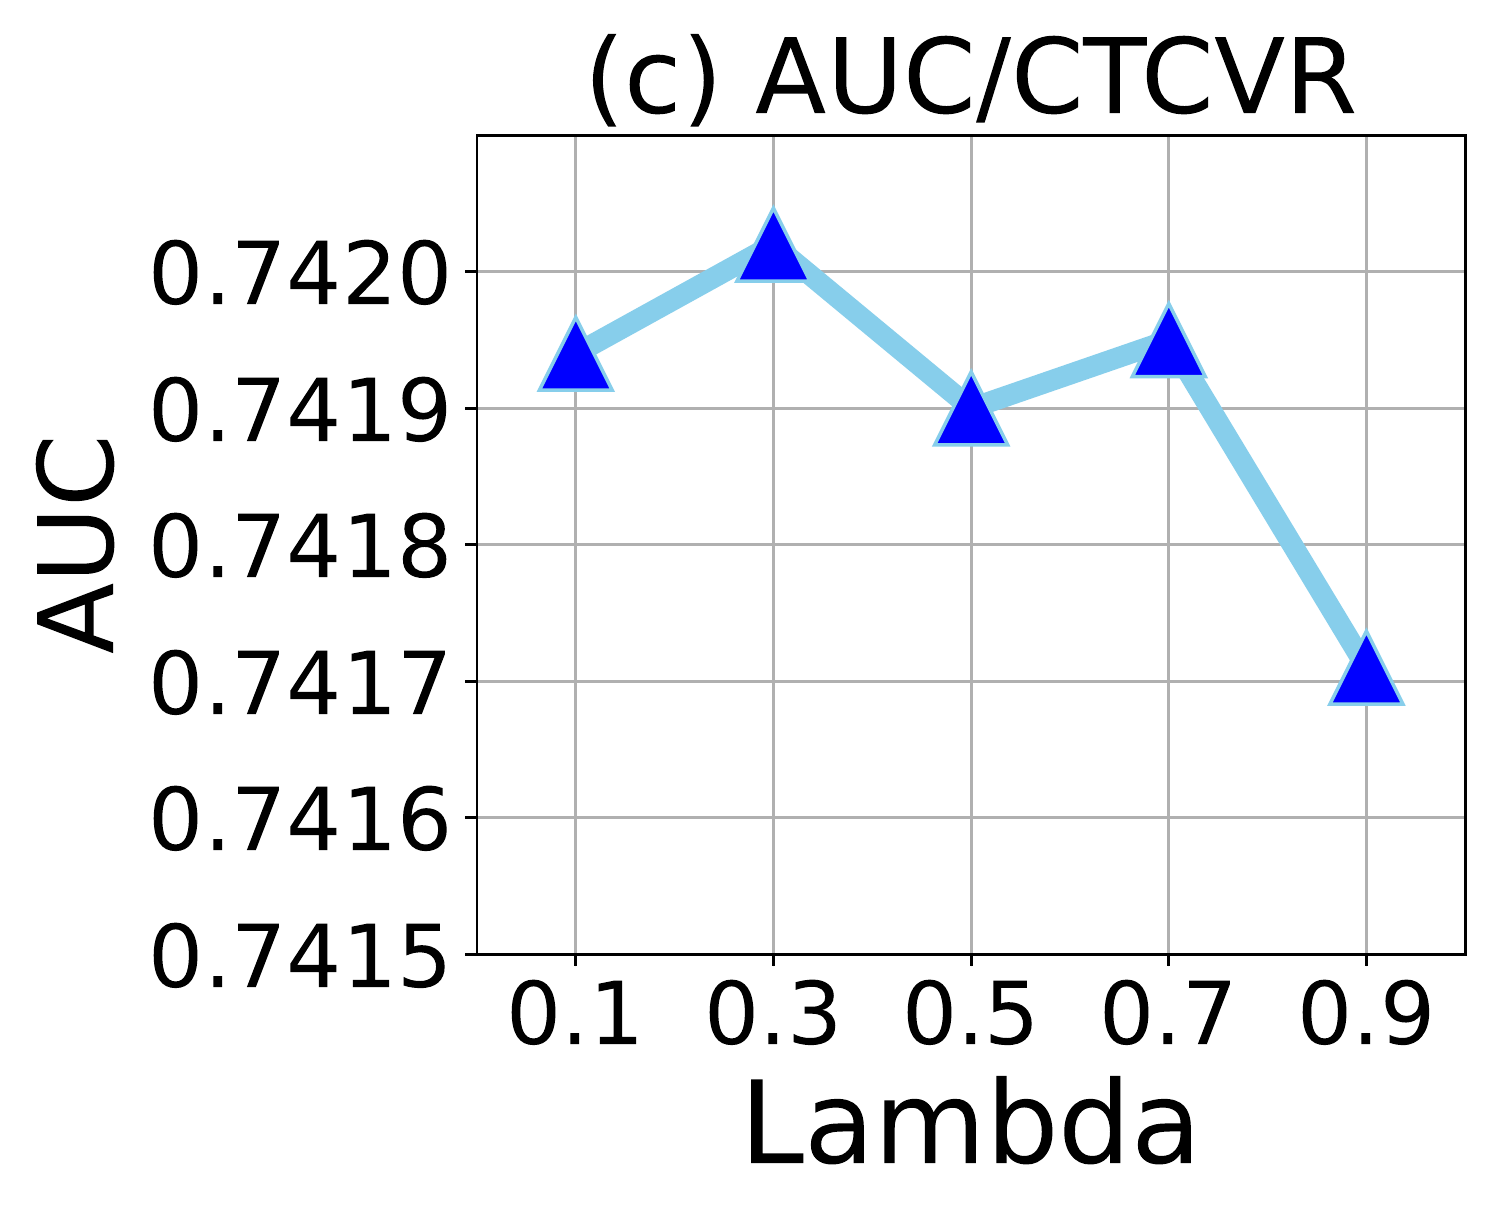}}}
	%	\hspace*{-0.6cm}
	{\subfigure{\includegraphics[width=0.48\linewidth]{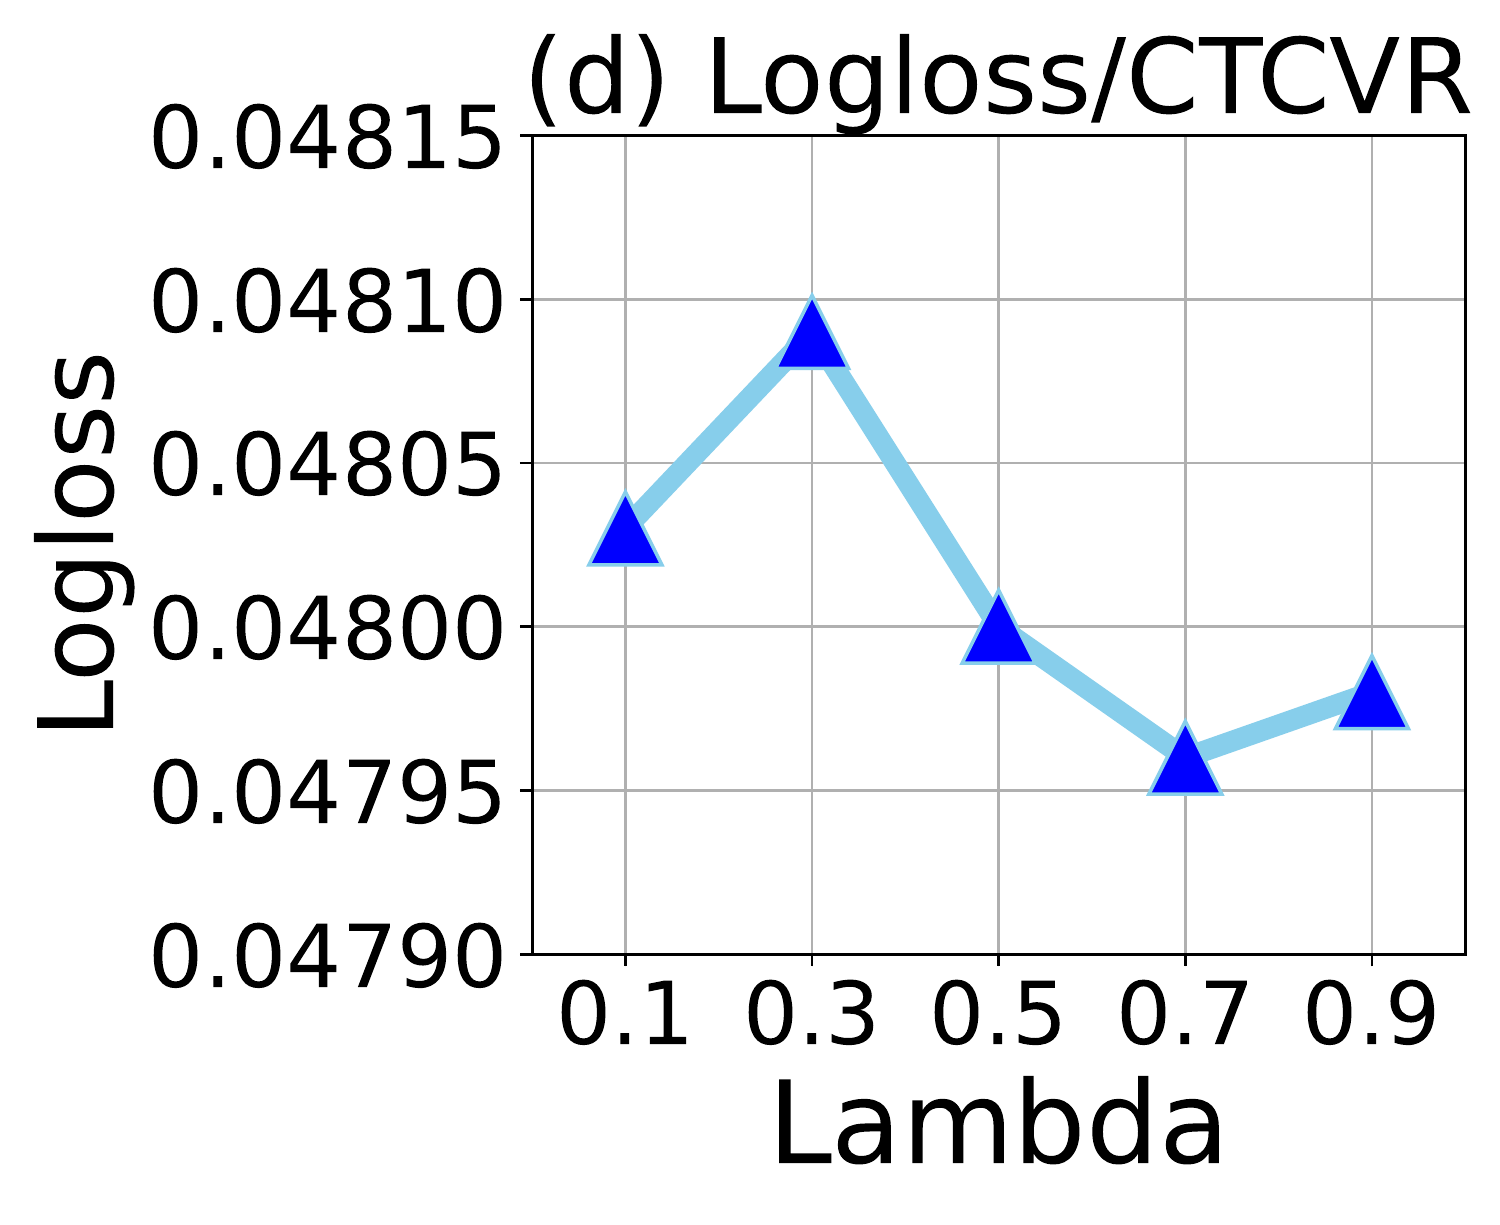}}}
	\caption{Parameter analysis for $\lambda$}\label{fig:Fig4}
	\vspace{-4.9mm}
\end{figure}

\begin{table}[h]
        \small
	\caption{Parameter analysis for $\alpha^{\theta}$}
	\label{table:C1}
	\begin{tabular}{@{}|c|c|ccccc|@{}}
		\toprule[1pt]
		\multirow{3}{*}{Task} & \multirow{3}{*}{Metric} & \multicolumn{5}{c|}{$\alpha^{\theta}$}\\ 
            \cmidrule(l){3-7} 
		&  & 5E-02 & 1E-02 & 5E-03 & 1E-03 & 5E-04 \\ \midrule

            \multirow{2}{*}{CTR} 
		& AUC $\uparrow$ & 0.73328 & \textbf{0.73417*} & 0.73416 & 0.73396 & 0.73390 \\
		& Logloss $\downarrow$ & 0.20158 & \textbf{0.20100*} & 0.20138 & 0.20130 & 0.20143 \\ \midrule

            \multirow{2}{*}{CTCVR} 
		& AUC $\uparrow$   & 0.74194 & 0.74201 & 0.74179 & \textbf{0.74208*} & 0.74177 \\
		& Logloss $\downarrow$ & \textbf{0.04790*} & 0.04798 & 0.04791 & 0.04800 & 0.04805 \\ \bottomrule[1pt]
	\end{tabular}
	\\ ``\textbf{{\Large *}}'' and \textbf{Bold} indicates the best performance of that row.
        \\ $\uparrow$: the higher the better; $\downarrow$: the lower the better.
		\vspace{-3mm}
\end{table}

\begin{table}[h]
        \small
	\caption{Parameter analysis for $\alpha^{\phi}$}
	\label{table:C2}
	\begin{tabular}{@{}|c|c|ccccc|@{}}
		\toprule[1pt]
		\multirow{3}{*}{Task} & \multirow{3}{*}{Metric} & \multicolumn{5}{c|}{$\alpha^{\theta}$}\\ 
            \cmidrule(l){3-7} 
		&  & 5E-02 & 1E-02 & 5E-03 & 1E-03 & 5E-04 \\ \midrule

            \multirow{2}{*}{CTR} 
		& AUC $\uparrow$ & 0.73358 & 0.73366 & 0.73370 & 0.73396 & \textbf{0.73413*} \\
		& Logloss $\downarrow$ & 0.20166 & 0.20171 & 0.20160 & \textbf{0.20130*} & 0.20183 \\ \midrule

            \multirow{2}{*}{CTCVR} 
		& AUC $\uparrow$   & 0.74157 & 0.74179 & 0.74132 & \textbf{0.74208*} & 0.74166 \\
		& Logloss $\downarrow$ & 0.04798 & \textbf{0.04788*} & 0.04817 & 0.04800 & 0.04789 \\ \bottomrule[1pt]
	\end{tabular}
	\\ ``\textbf{{\Large *}}'' and \textbf{Bold} indicates the best performance of that row.
        \\ $\uparrow$: the higher the better; $\downarrow$: the lower the better.
		\vspace{-3mm}
\end{table}

\end{appendix}
